# Supplementary material for: Phone2Proc: Bringing Robust Robots Into Our Chaotic World
Source: arXiv:2212.04819 source file (2022-12-08)
Supplement: Supplementary file 1 [file 00_supp.tex]

\documentclass[10pt,twocolumn,letterpaper]{article}

\usepackage[review]{cvpr}      %

\usepackage{graphicx}
\usepackage{amsmath}
\usepackage{amssymb}
\usepackage{booktabs}

\usepackage{multirow}
\usepackage{enumerate}
\usepackage{color}
\usepackage{xspace}
\usepackage{booktabs}
\usepackage{makecell}

\usepackage{enumitem}

\usepackage[pagebackref,breaklinks,colorlinks]{hyperref}

\usepackage[capitalize]{cleveref}
\crefname{section}{Sec.}{Secs.}
\Crefname{section}{Section}{Sections}
\Crefname{table}{Table}{Tables}
\crefname{table}{Tab.}{Tabs.}

\usepackage{xcolor}
\definecolor{myblue}{HTML}{226DA3}
\hypersetup{
    citecolor=myblue
}

\begin{document}

\title{Phone2Proc: Bringing Robust Robots Into Our Chaotic World\\Supplementary Material}

\author{First Author\\
Institution1\\
Institution1 address\\
{\tt\small firstauthor@i1.org}
\and
Second Author\\
Institution2\\
First line of institution2 address\\
{\tt\small secondauthor@i2.org}
}

\maketitle
\appendix
\input{07_supplementary}

{\small
\bibliographystyle{ieee_fullname}
\bibliography{egbib}
}

\end{document}
